# Supplementary material for: Piracy Resistant Watermarks for Deep Neural Networks
Source: arXiv:1910.01226 source file (2020-12-02)
Supplement: Supplementary file 1 [file revision_appendix.tex]

\clearpage
\section{Modification based on ``Concerns to be Addressed in MR''}
We thank all the reviewers for their constructive comments. We have followed the reviews to modify the paper
accordingly. In the following, we begin by presenting our response to
each of the six items listed in the ``concerns to be addressed in MR''
section of the review.  Later in Appendix C we present the detailed
response to comments raised by each individual reviewer.

% As requested, we respond to reviewer concerns in this letter. We
% begin by addressing the primary concerns noted by the reviewers
% in their reject and resubmit decision. All these concerns have
% been addressed in our paper, and we expound further upon them
% here. The exact text of the reviewers' statements are in the bold headings, and our response is
% below.

\vspace{0.05in} \noindent 1. {\em A more comprehensive evaluation of model extraction; the
  reviewers are not fully convinced by the authors' argument for it
  being out of scope here (specifically, please see comments from
  Rev. D).}

\para{A:} We took this suggestion and added additional results on model
extraction in \S\ref{subsec:stealing}. Our conclusion is that with
significant data and computation resources, it is possible to perform the
attack, but it provides limit benefit. Of the main challenges to training a
proprietary model (getting in-distribution data, labeling it, and costs of
training the model), a successful extraction attack addresses 1 of the 3.  We
quantified the magnitude of the remaining 2 and present the results in the
revision in \S\ref{subsec:stealing}.
%\forben{}\fixme{add more text on model extraction conclusion} 

% Specifically, we show that our
% watermark system can be combined with an existing
% defense~\cite{jia2020entangled}, which is designed explicitly to
% defend against model
% extraction attacks. We present evaluation results of the combined
% system in \S\ref{subsec:stealing}, which
% show that \forben{} \fixme{summary of performance.}

% To defend against model extraction, we combine our system with that
% of~\cite{jia2020entangled}. This watermark method was designed explicitly
% to defend against model extraction. \S\ref{sec:countermeasure}
% explores the performance of this combined system. \todo{is this enough?}

\vspace{0.05in} \noindent 2. {\em  Evaluation of algorithm performs using some other
  classification task (e.g., speech recognition), or, alternatively,
  understand if it only works in the image domain and why. (Rev. C)}

\para{A:}  We follow the suggestion and add two non-image 
classification tasks to our evaluation:   speech recognition
(recognizing digits 0-9 from .wav audio files),  human activity
recognition using accelerometer data from the WISDM
dataset.  We add description of the two tasks (their model architectures and datasets) in \S\ref{sec:expr_setup} and
Tabel~\ref{table:dataset}, and add the results of the watermark experiments on
both.  Overall, they show the same conclusion as
the existing tasks.

We also add text in the beginning of \S\ref{sec:intuition} to explain
how our image-based design can be applied to these two new non-image tasks.

% \forben{need this?} Furthermore, as our watermark design and evaluation target
% CNN models, we add text in\S\ref{subsec:threat} to
% clarify this context.

% We have added two additional tasks to our evaluation: speech
% recognition and human activity recogntion. These tasks are described
% in~\S\ref{sec:eval}, and our watermark performance on these tasks is
% illustrated throughout the paper.

\vspace{0.05in} \noindent 3. {\em  Adapting Neural Cleanse for the specific watermark patterns
  introduced by the defense and/or evaluation of an attack that
  specifically looks for extreme values introduced by watermarking (as
  mentioned by Rev. B, Rev. D, Rev. E), and adding results from
  evaluations of Fine-pruning and ABS.}

\para{A:} Thank you. We followed the suggestion and added results for ABS and
fine pruning, as well as an optimized version of NeuralCleanse in
\S\ref{subsec:backdoor_detection}. First, we consulted with original authors of
NeuralCleanse, and adapted its search range to include the extreme values
used by our watermark (assuming that the attacker knows the exact $\lambda$
used to construct the watermark). We refer to the result as
NeuralCleanse++. Our result in Table~\ref{table:neural_cleanse} shows that
NeuralCleanse++ is unable to detect the presence of our proposed watermark in
models.  Although a small portion (6 out of 50) of watermark models have
anomaly index above 2 detected by NeuralCleanse++, even more watermark-free
models (11 out of 50) are also flagged as anomalies. In addition, for each of
the watermarked models marked as anomalies, NeuralCleanse++ identifies the
wrong target labels.

We also add detailed results of using fine-pruning and ABS to detect and
remove backdoors in \S\ref{subsec:backdoor_detection}.  ABS detects zero
anomalies across all our models (both watermarked and watermark-free). For
fine pruning, our watermarks for all tasks survive fine-pruning despite
testing with a broad range of pruning ratios (from 10\% to 70\%). We present
the detailed results of these experiments in Figure~\ref{fig:fine_pruning}.

% We made the requested adaptations to NeuralCleanse. In our adaptation,
% we assume the attacker knows $\lambda$, the extreme value used in
% watermark construction. As shown in~\S\ref{sec:countermeasure}, even
% with this adaptation NeuralCleanse is unable to detect our
% watermark. Results from fine-pruning and ABS are also included
% in~\S\ref{sec:countermeasure}. Both methods fail to detect our
% watermark.

\vspace{0.05in} \noindent 4. {\em  Report results against several instantiations with an
  average and error bars to understand the variation in the expected
  results. (Rev. C and Rev. D)}

\para{A:}  For all the experiments, we now present results as average and standard deviation across multiple runs for all
  the experiments. These include Table~\ref{table:prework_piracy_std}, \ref{table:performance},
\ref{table:verification_overhead}, \ref{table:tl_normal_acc},
\ref{table:tl_wm_acc}, \ref{table:neural_cleanse}, \ref{tab:substitute}, 
\ref{table:piracy},  and Figure~\ref{fig:piracy_bar},
\ref{fig:fine_tuning}, \ref{fig:pruning}, \ref{fig:fine_pruning}.
Figure~\ref{fig:overhead} plots all the result data points across 
the experiments. 

We did not include average/std results in
Figure~\ref{fig:acc_change_percent}, since this figure is an illustrative
example of a single instance to demonstrate the concept.

%is to show an example on the model performance for the same pirate watermark, we do not report the average results for multiple
%runs.  We also add text to discuss the observed
%variation in these results.}
% where each run uses a model injected with a randomly
% chosen ownership watermark.

% All results reported in the paper now represent an average across 10 runs
% of the given experiment. Where possible and/or appropriate, we have included
% error bars in our graphs.

\vspace{0.05in} \noindent 5. {\em  Results on the computational costs and overheads of
  watermarking (Rev. E)}

\para{A:}     In~\S\ref{subsec:overhead}, we add new results on the
computation costs of injecting and verifying our proposed watermark
design, Figure~\ref{fig:overhead} for injection
and  Table~\ref{table:verification_overhead} for verification. 

A quick summary of results:  for watermark injection, we show that
training a watermarked model requires computation time that is
comparable to that of training a watermark-free model.  For all six
tasks, a watermarked
model can achieve more than 95\% of normal classification accuracy
after using 115\% of training time for watermark-free models.

Verification of a watermark takes $\sim 1s$ for all six tasks, when we
use 1,000 test samples.  This achieves the same verification decision
as if we use all test data for verification (listed in Table~\ref{table:dataset}). 
% or injection, the watermarked models can achieve over 95\% of the average normal classification accuracy with
% in 115\% of the average training time for WM-free models for all tasks. For verification, we find that we can use
% 1,000 samples to do verification in $\sim 1s$ for all tasks without
% degrade the watermark verification process.

Overall, these
results suggest that our watermark design incurs reasonable overheads
in both watermark 
injection and verification. 

%We have collected these metrics and have included them
%in~\S\ref{sec:eval}. \todo{Is this where they are?}

\vspace{0.05in} \noindent 6. {\em  In addition, please make all editorial and typographical
  changes suggested by the reviewers.}

\para{A:}  Thank you for all the detailed comments. We follow the reviews and make changes to our
text accordingly.  In particular, we replace each task's name by the dataset name;
update the text to replace any gender reference to the general
they/their reference; and change the term ``training cycles'' to
``training batches'' to make it more intuitive.

% We use the dataset name rather than rename it for task name,
% update the text to avoid making assumptions about the adversary's gender,
% change "training cycles" to "training batches" to make it clearer.

Finally, our modifications are marked in \revision{this color}.

%We have incorporated these suggestions. Thank you.
