# Supplementary material for: Piracy Resistant Watermarks for Deep Neural Networks
Source: arXiv:1910.01226 source file (2020-12-02)
Supplement: Supplementary file 2 [file response_appendix.tex]

\newpage
\section{Response to Detailed Reviewer Comments}

% Next, we address other concerns raised by reviewers which were not
% indicated as strictly necessary to the major revision (and which were
% not addressed in the points above). The concerns raised by each
% individual are listed below, followed by our response.

We present our response to any individual review comments not
already included in Appendix B.  Again, we thank the reviewers
for their helpful comments to improve this paper. 

\subsection*{Reviewer A}
\noindent {\em Did not compare results to existing
  methods.}

\para{A:}  We have added text (in \S\ref{subsec:evalpirate} and
\S\ref{subsec:evalbasic})  to strengthen the connection between the
evaluation results on 
existing methods (in \S\ref{sec:piracy}) and the results on
our watermark method in \S\ref{sec:eval}.   


\vspace{0.05in} \noindent  {\em Did not address distillation attacks.}

\para{A:} Thank you for this note. We did in fact do extensive experiments to
test the impact of distillation on our watermarks. What we found was
surprising, that prior claims of distillation as a way to train models using
smaller datasets was overblown. Our results suggest those earlier conclusions
were due to a high level of redundancy in training data, which when reduced,
seemed to suggest a concrete benefit to distillation where they were none. In
our repeatedly tests, we could consistently train accurate models from
scratch, using training sets produced by distillation. This means
distillation as an attack provides no additional benefit to attackers over
training a model from scratch. We feel like these conclusions are tangential
to the focus of our paper, so we put them into the appendix. We plan on
exploring this result further in a separate followup paper.

% As we have discussed during
% the rebuttal phase, we did evaluate our watermark against distillation
% attacks, where we use a substitute dataset to train a smaller
% distilled model. The results were very similar to those of the model
% extraction attack analysis.  \forben{}  \fixme{Thus we add text in 
%   \S\ref{subsec:stealing} to state the similarity of distillation and
%   model extraction attacks and add its results to the Appendix??} 

% \huiying{ Prior work argues that distillation attacks can train accurate models
% using smaller datasets (compared to datasets used to train models from scratch).
% However, we find that this is somewhat misleading. We use 20\% of the training data
% for \mnist{} and \cifar{} to train a model from scratch as well as train a model
% using distillation. We find that the improvements via distillation is negligible for
% both tasks. For \mnist{}, the normal classification accuracy is 95.3\% training from
% scratch while 95.5\% using distillation; for \cifar{}, the normal classification accuracy is 77.6\% training from
% scratch while 79.3\% using distillation. Thus, we chose not to address distillation attacks given their remarkable similarity to
% model extraction attacks.
% }


\subsection*{Reveiwer B}

\vspace{-0.05in} \noindent  {\em How about using an extremely small learning rate to
  inject pirate
  watermark.}

\para{A:} This is a great suggestion.  We ran piracy attack
experiments against our watermarks by using very small learning
rates.  We found that while a smaller learning rate does help the
attacker to improve normal classification accuracy,  but the attacker
still cannot embed the pirate watermark or erase the original (owner)
watermark. We have added text to \S\ref{subsec:evalpirate} to explain this
observation. 

% For example, our experimented on \mnist{} using small learning
% rates ($5\cdot 10^{-4}$, $10^{-4}$, $10^{-5}$, $10^{-6}$) to embed a
% randomly chosen pirate watermark (repeated 100 runs).   Using a very
% small learning rate ($10^{-5}$, $10^{-6}$), the piracy attack can
% achieve a normal classification accuracy in the range of 91\%-95\%,
% but the classification accuracy for the pirate watermark is only
% 13\%-19\%, and the classification accuracy for the owner watermark is
% still 85\%-94\%.  This means that a piracy attack using a very small
% learning rate cannot embed the pirate watermark or erase the owner
% watermark.   \fixme{\bf We added text in XXXXX to explain this
%   observation}

% Thank you for this suggestion. We ran several piracy attacks against
% our watermarking system in which the attacker used a very small
% learning rate. We found that a smaller learning rate allows the
% attacker to better maintain normal model accuracy. However, the attacker still cannot
% successfully embed a pirate watermark with this parameter
% modification. \huiying{Specifically, we run experiments on \mnist~ using different learning rate
% ($5e-4, 1e-4,1e-5,1e-6$) to embed the pirate watermarks (for each learning rate we run 100
% different pirate watermarks), we find that $1e-5$ and $1e-6$ could maintain average normal classification
% accuracy at a level of 91\% and 95\%, but the corresponding average watermark accuracies for owner's watermark are
% 85\% and 94\%, while the corresponding average watermark accuracies for pirate watermarks are just 13\% and 19\%.}

\subsection*{Reviewer C}
\vspace{0.05in} \noindent  {\em Unclear how many additional training samples are required.}

\para{A:}  Thank you for noting this. We have added clarifying text
in~\S\ref{sec:expr_setup}. 


\vspace{0.05in} \noindent  {\em Table~\ref{table:piracy} shows $> 0\%$ values for pirate
  WM. Why?}

\para{A:} The presence of non-zero values comes from a classifier
model's propensity to randomly guess a class, leading to an accuracy
level of $1/N$ where $N$ is the number of classes.   The pirate
watermark's classification results in  Table~\ref{table:piracy}
closely approximate this result.  Furthermore, since these values are
much lower than the verification threshold  $T_{watermark}$, these
pirate watermarks will not be verified.  We added text in
\S\ref{subsec:evalpirate} to clarify this point.  


% The appearance of non-zero values for the pirate WM is due to the model's propensity to randomly guess a
% class for out-of-domain inputs. Since the pirate WM is unknown
% to the model, the model will randomly place it into one of its $N$
% classes. Over many trials, we expect the pirate
% watermark to have an average accuracy of $1/N$. For each class, the
% piracy results in Table~\ref{table:piracy} approximate this expected
% value. Since $1/N$ is far below the verification threshold $T_{watermark}$,
% this phenomenon will not affect piracy-resistance.
% \fixme{TODO: add a short sentence to explain that in the text.}

\vspace{0.05in} \noindent  {\em Table \ref{table:neural_cleanse} shows Neural Cleanse anomalies for face/traffic
  models. Why?} 

\para{A:}  Thank you for pointing this out. We have added text 
in \S\ref{subsec:backdoor_detection} to explain why some models'
anomaly values are above 2.   We also added a customized Neural
Cleanse version to detect extreme values in the input, showing it is
still ineffective. 

\vspace{0.05in} \noindent  {\em Table~\ref{tab:substitute_tramer} is missing values for ImageNet and Random at 376K
  training images.}

\para{A:} We have added these numbers. 

\subsection*{Reviewer D}

\noindent  {\em Piracy evaluation assumes the adversary will follow the
  same watermarking procedure.}

\para{A:}  Yes, we assume the adversary follows the same
watermarking procedure as the owner. The owner can publicly announce
their chosen watermark scheme upon licensing their model. Thus, anyone
hoping to claim ownership over this model must construct a pirate
watermark using the announced procedure.   We added text in
\S\ref{subsec:threat} to explain this assumption.

\noindent {\em The word inexorably is strong on the 2nd page in the
  introduction.}

\para{A:} We removed this word from the introduction.

 \vspace{0.05in} \noindent  {\em Given that most deep neural network
   training procedures are not deterministic, it would help to clarify
   what deterministic refers to in the following sentence: "The entire
   recovery process is transparent and deterministic, and can be
   audited by an honest third party. "}

 \para{A:} Yes, the word deterministic here is misused. We have removed it
 from the sentence.

\subsection*{Reviewer E}
\noindent  {\em Claim of being the “first piracy resistant watermarking
  method” is unjustified.}

\para{A:}  We very much appreciate the comment. To justify our claim, we
improved \S\ref{sec:back} and \S\ref{sec:piracy} to provide more
information on why existing designs fail to provide piracy
resistance.   In particular, we added text to explain why
DAWN~\cite{szyller2019dawn} fails to provide piracy resistance.  The
other work \cite{darvish2019deepsigns} mentioned in the review is
already discussed in the paper (as an existing watermark design that
fails to resist piracy attacks). 




% As far as we can tell, there is no watermarking method that claims that they can
% resist against piracy attacks. DeepSigns, the first work mentioned by
% the reviewer (\cite{darvish2019deepsigns}) was indeed addressed in our
% paper (see Section~\ref{sec:piracy}). As we
% noted,~\cite{wang2019attacks} has already shown that regularizer-based
% watermarks like DeepSigns are vulnerable to piracy
% attacks.
% DAWN (\cite{szyller2019dawn}) has a unique threat model that requires
% explanation before we can explore its piracy resistance.
% Due to its black-box scenario, DAWN does not actually watermark a
% proprietary model. It instead modifies a subset of
% query responses returned by that model. When an attacker uses these
% modified sampels to train a new model (via a model extraction attack),
% they leave a detectable ``mark'' inside the new model. This ``mark'' is the watermark
% they refer to, and it can be used to prove that the attacker's model
% was indeed stolen.

% In this context, piracy-resistance means that the ``mark'' in the new
% model is indisputable, a property DAWN cannot guarantee. While DAWN
% finds that an adversary cannot detect or remove the mark, it provides
% no analysis of whether an attacker can insert an {\em additional} mark to
% dispute model ownership. It would be trivially possible for an
% adversary to pre-register many ``marks'' of their own (since the mark is
% not model-dependent) and train at least one into the pirated
% model. DAWN states (in Appendix F) that if $>1$ watermark is found in
% a model, ownership will default to the mark that was registered first. If the attacker
% registers their mark before the true owner registers theirs, the
% attacker succeeds in pirating the emodel. Because this crucial aspect of
% piracy-resistance goes unaddressed in this paper, it cannot be
% ascertained that DAWN is indeed piracy resistant. Our
% claim stands.

\vspace{0.05in}\noindent  {\em Watermarking method is not applicable to existing models
  due to the necessity of null-embedding.}

\para{A:}   This is true. Our work is designed to protect {\em
  unreleased} models, not
ones that have already been distributed to external parties. We stated
this in \S\ref{sec:discussion} as one of the limitations. 

%Once an unwatermarked model is released publicly, it is
%instantly vulnerable to piracy, theft, and other attacks. Even if we could use our%
%method to watermark existing models, it (or any watermark
%system) would be unable to repair past damage.
